# Supplementary material for: ViSAGe: Video-to-Spatial Audio Generation
Source: arXiv:2506.12199 source file (2025-06-13)
Supplement: Supplementary file 1 [file table_additional_result.tex]

\begin{table*}
\caption{Results on YT-Ambigen. V2A denotes video-to-audio generation. CS and Corr refer to the CAVP score and correlation coefficient, respectively. PT, DIR, PE, and RA stand for pretraining, directional embedding, patchwise energy map, and rotation augmentation, respectively.}
\label{table:yt-ambigen}
\centering
\resizebox{\textwidth}{!}{
\begin{tabular}{cccccccccccccc}
\hline

\multicolumn{4}{c}{Model} & \multicolumn{3}{c}{Semantic Metrics} & \multicolumn{7}{c}{Spatial Metrics} \\

\multicolumn{2}{c}{\multirow{2}{*}{V2A}} & \multicolumn{2}{c}{\multirow{2}{*}{Spatialization}} & \multirow{2}{*}{FAD\textsubscript{m $\downarrow$}} & \multirow{2}{*}{KLD\textsubscript{m $\downarrow$}} & \multirow{2}{*}{CS \textsubscript{m $\downarrow$}} & \multirow{2}{*}{FAD\textsubscript{avg $\downarrow$}} & \multicolumn{3}{c}{AUC\textsubscript{$\uparrow$}} & \multicolumn{3}{c}{Corr\textsubscript{$\uparrow$}} \\

& & & & & & &  & All& 1fps & 5fps & All& 1fps & 5fps \\
\hline

\multicolumn{14}{c}{\textbf{Comparison to baseline models}} \\

\multicolumn{2}{c}{\multirow{2}{*}{SpecVQGAN}} & \multicolumn{2}{c}{Ambi Enc.} & 4.61  & 2.24 &   & \textbf{4.17} & 0.687 & 0.680 & 0.670 & 0.349 & 0.337 & 0.322  \\

& & \multicolumn{2}{c}{Audio Spatial.} & 5.00 & 2.50  & & & & & & & & \\

\multicolumn{2}{c}{\multirow{2}{*}{Diff-foley}} & \multicolumn{2}{c}{Ambi Enc.} & 5.68 & 2.60 & & 5.53 & 0.687 & 0.680 & 0.670 & 0.349 & 0.337 & 0.322 \\

& & \multicolumn{2}{c}{Audio Spatial.} & 7.24 & 2.51 & & 8.76 & 0.826 & 0.803  & 0.777 & 0.577 & 0.537 & 0.494 \\

\multicolumn{4}{c}{ViSAGe} & \textbf{3.86} & \textbf{1.71} & & 4.20  &\textbf{0.846} & \textbf{0.819} & \textbf{0.790}& \textbf{0.635} & \textbf{0.584} & \textbf{0.531}\\
\hline

\multicolumn{14}{c}{\textbf{Ablation on Model Components}} \\

\textbf{PT} & \textbf{DIR} & \textbf{PE} & \textbf{RA} & & & & & &  & & & & \\

\cmark &  & & & \textbf{3.73} & 1.76 & & 4.19& 0.724 & 0.708 & 0.689 & 0.430 & 0.398 & 0.362 \\

\cmark & \cmark & & & 3.74 & 1.77 & & \textbf{4.04} & 0.778 & 0.757 & 0.734 & 0.524 & 0.482 & 0.439 \\

& \cmark & \cmark &  & 5.24 & 1.97  & & & 0.788 & 0.762 & 0.736 & 0.536 & 0.485 & 0.435 \\

\cmark & \cmark & \cmark & & 4.01  & 1.78 & & 4.30 & 0.782 & 0.759 & 0.735 & 0.531 & 0.486 & 0.441 \\

\cmark & \cmark & \cmark & \cmark & 3.86 & \textbf{1.71} & & 4.20 &\textbf{0.846} & \textbf{0.819} & \textbf{0.790}& \textbf{0.635} & \textbf{0.584} & \textbf{0.531}  \\ 
\hline

\multicolumn{14}{c}{\textbf{Ablation on Code Generation Pattern}} \\
\multicolumn{4}{c}{Sequential Delay} & 10.75 & 2.66 & & & 0.746 & 0.716  & 0.695 & 0.386  & 0.341 & 0.311 \\
\multicolumn{4}{c}{Residual Only} & 4.68 & 1.97 & & 4.37 & 0.777 & 0.759 & 0.738 & 0.480 & 0.448 & 0.413 \\
\multicolumn{4}{c}{Spatial Only} & 5.89 & 2.01 & & 5.69 & 0.779 & 0.756 & 0.732 & 0.511 & 0.468 & 0.425 \\
\multicolumn{4}{c}{Ours} & 5.24 & 1.97 & & 4.96 & 0.788 & 0.762 & 0.736 & 0.536 & 0.485 & 0.435 \\
\hline
\multicolumn{14}{c}{\textbf{Ablation on Classifier-Free Guidance}} \\
\multicolumn{4}{c}{Visual \& Directional} & 3.86 & \textbf{1.71} & & 4.20 & 0.846 & 0.819 & 0.790& 0.635 & 0.584 & 0.531  \\ 
\multicolumn{4}{c}{Visual Only} & \textbf{3.85} & \textbf{1.71} & & \textbf{4.14} & 0.757 & 0.736 & 0.716 & 0.488 & 0.446 & 0.406 \\
\multicolumn{4}{c}{Directional only} & 5.56 & 2.01 & & 4.76 & \textbf{0.890} & \textbf{0.864} & \textbf{0.839} & \textbf{0.721} & \textbf{0.671} & \textbf{0.624} \\
\multicolumn{4}{c}{Dual 2.5 \& 2.5} & 3.93 & 1.72 & & 4.22 & 0.795 & 0.772 & 0.748 & 0.549 & 0.505 & 0.459 \\
\multicolumn{4}{c}{Dual 2.5 \& 7.5} & 4.32 & 1.76 & & 4.59 & 0.829 & 0.798 & 0.769 & 0.596 & 0.540 & 0.487 \\
\hline

\end{tabular}
}
\end{table*}
